# Supplementary material for: Reference Energies for Intramolecular Charge-Transfer Excitations
Source: arXiv:2103.02947 source file (2021-04-12)
Supplement: Supplementary file 1 [file CT-SI.pdf]

# Reference Energies for Intramolecular Charge-Transfer Excitations Supporting Information

Pierre-François Loos,[†] Massimiliano Comin,[‡] Xavier Blase,[‡] and Denis Jacquemin[¶]

†*Laboratoire de Chimie et Physique Quantiques, Université de Toulouse, CNRS, UPS, France*

‡*Univ. Grenoble Alpes, CNRS, Inst NEEL, F-38042 Grenoble, France*

¶*Université de Nantes, CNRS, CEISAM UMR 6230, F-44000 Nantes, France*

E-mail:

# S1 Additional data and key MOs

Below are additional data obtained for the various investigated CT transitions, together with the representation of the key MOs. Note that we used LR-CCSD/cc-pVTZ as reference, so that the oscillator strength ($f$) given are obtained at this level of theory, as are the state numbering and the MO composition (the represented MOs are HF/cc-pVTZ). The extra values given for TD-CAM-B3LYP and ISR-ADC(2) use the same atomic basis set, but the state numbering is not necessarily the same for all levels of theory.

Table S1: Extra data for the investigated states. The transition energies are in eV, the CT distances in Å, and the CT charge in $e$. All values have been obtained with the cc-pVTZ basis set.

| | | | LR-CCSD | | | TD-CAM-B3LYP | | | | ISR-ADC(2) | | |
|---|---|---|---|---|---|---|---|---|---|---|---|---|
| Compound | State | Sym | $\Delta E$ | $f$ | MO combination | $\Delta E$ | $f$ | $d^{CT}$ | $q^{CT}$ | $\Delta E$ | $f$ | $r^{eh}$ |
| Aminobenzonitrile | $S_2$ | $A_1$ | 5.408 | 0.447 | 31-32 (-0.637) | 5.212 | 0.414 | 1.154 | 0.352 | 5.158 | 0.518 | 1.006 |
| Aniline | $S_3$ | $A_1$ | 5.985 | 0.175 | 25-29 (-0.613); 24-26 (+0.254) | 5.767 | 0.134 | 1.020 | 0.295 | 5.788 | 0.244 | 0.827 |
| Azulene | $S_2$ | $A_1$ | 4.018 | 0.003 | 34-36 (-0.489); 33-35 (-0.457) | 3.753 | 0.003 | 1.164 | 0.236 | 3.859 | 0.004 | 1.064 |
| | $S_3$ | $B_2$ | 4.824 | 0.055 | 33-36 (-0.573); 32-35 (-0.286) | 4.795 | 0.075 | 1.023 | 0.332 | 4.670 | 0.063 | 0.953 |
| Benzonitrile | $S_5$ | $A_2$ | 7.329 | | 25-28 (-0.606) | 6.617 | | 1.170 | 0.731 | 7.285 | | 1.183 |
| Benzothiadiazole | $S_2$ | $B_2$ | 4.634 | 0.058 | 35-36 (0.656) | 4.150 | 0.056 | 1.414 | 0.427 | 4.456 | 0.075 | 1.239 |
| DMABN[a] | $S_2$ | $A_1$ | 5.100 | 0.585 | 39-40 (0.641) | 4.964 | 0.548 | 1.477 | 0.407 | 4.727 | 0.616 | 1.439 |
| Dimethylaniline | $S_1$ | $B_2$ | 4.657 | 0.042 | 33-34 (-0.611); 32-36 (-0.257) | 4.742 | 0.053 | 1.127 | 0.484 | 4.469 | 0.051 | 0.978 |
| | $S_2$ | $A_1$ | 5.680 | 0.319 | 33-36 (0.630) | 5.529 | 0.262 | 1.253 | 0.370 | 5.348 | 0.386 | 1.219 |
| Dipeptide | $S_{12}$ | $A''$ | 8.924 | 0.000 | 33-39 (0.556); 33-41 (0.288) | 7.841 | 0.000 | 2.165 | 1.295 | 7.823 | 0.000 | 3.617 |
| $\beta$-Dipeptide | $S_{15}$ | $A'$ | 8.899 | 0.017 | 39-43 (0.494); 38-43 (-0.241) | 8.011 | 0.002 | 2.357 | 1.048 | 8.299 | 0.004 | 3.155 |
| | $S_{17}$ | $A''$ | 9.575 | 0.000 | 37-43 (-0.587); 37-46 (0.215) | 8.376 | 0.009 | 2.292 | 1.028 | 8.448 | 0.001 | 4.348 |
| Hydrogen Chloride | $S_{1/2}$ | $\Pi$[b] | 8.175 | 0.218 | 8/9-10 (-0.661) | 7.829 | 0.226 | 1.047 | 0.711 | 8.303 | 0.239 | 0.954 |
| Nitroaniline | $S_4$ | $A_1$ | 4.804 | 0.410 | 36-37 (-0.650) | 4.473 | 0.371 | 2.021 | 0.558 | 4.436 | 0.443 | 2.081 |
| Nitrobenzene | $S_4$ | $A_1$ | 5.767 | 0.214 | 31-33 (0.638) | 5.221 | 0.211 | 1.660 | 0.559 | 5.555 | 0.260 | 1.512 |
| NDMA[c] | $S_2$ | $A_1$ | 4.529 | 0.511 | 44-45 (-0.651) | 4.252 | 0.458 | 2.184 | 0.589 | 4.047 | 0.509 | 2.410 |
| Nitropyridine N-Oxide | $S_4$ | $A_1$ | 4.464 | 0.422 | 36-37 (-0.644) | 4.264 | 0.371 | 1.696 | 0.401 | 3.618 | 0.446 | 1.972 |
| N-Phenylpyrrole | $S_3$ | $B_2$ | 5.843 | 0.017 | 37-39 (-0.650) | 5.353 | 0.015 | 2.106 | 0.676 | 5.573 | 0.014 | 2.128 |
| | $S_4$ | $A_1$ | 6.524 | 0.237 | 37-40 (0.619) | 5.999 | 0.185 | 2.277 | 1.030 | 6.065 | 0.206 | 3.544 |
| Phthalazine | $S_1$ | $A_2$ | 4.264 | | 32-35 (-0.603); 32-39 (0.269) | 4.044 | | 1.107 | 0.737 | 3.791 | | 1.874 |
| | $S_2$ | $B_1$ | 4.635 | 0.005 | 32-36 (0.635) | 4.393 | 0.004 | 1.126 | 0.726 | 4.225 | 0.003 | 1.872 |
| Quinoxaline | $S_3$ | $B_2$ | 5.002 | 0.034 | 34-35 (-0.647) | 4.566 | 0.036 | 1.507 | 0.554 | 4.649 | 0.043 | 1.755 |
| | $S_4$ | $A_1$ | 6.009 | 0.374 | 34-36 (0.411); 33-38 (-0.403) | 5.997 | 0.626 | 1.117 | 0.301 | 5.823 | 0.527 | 0.973 |
| | $S_8$ | $B_1$ | 6.868 | 0.003 | 32-38 (-0.624) | 6.549 | 0.003 | 1.210 | 0.755 | 6.253 | 0.002 | 1.851 |
| Twisted-DMABN[a] | $S_1$ | $A_2$ | 4.413 | | 38-40 (-0.645) | 3.982 | | 1.992 | 1.017 | 3.842 | 0.000 | 2.686 |
| | $S_3$ | $B_1$ | 5.193 | 0.000 | 38-41 (0.661) | 4.779 | 0.000 | 1.737 | 1.090 | 4.496 | 0.000 | 2.597 |
| Twisted-PP[d] | $S_2$ | $B_2$ | 6.100 | 0.001 | 38-40 (0.649) | 5.382 | 0.000 | 2.332 | 0.813 | 5.670 | 0.001 | 3.322 |
| | $S_3$ | $A_1$ | 6.176 | 0.008 | 38-39 (-0.583) | 5.618 | 0.030 | 2.377 | 1.100 | 5.820 | 0.025 | 3.322 |
| | $S_4$ | $A_2$ | 6.351 | | 37-40 (0.637) | 5.944 | | 2.319 | 1.042 | 5.902 | 0.000 | 3.268 |
| | $S_5$ | $B_1$ | 6.614 | 0.008 | 37-39 (0.573) | 6.191 | 0.001 | 2.368 | 0.993 | 6.127 | 0.001 | 3.367 |

[a]Dimethylaminobenzonitrile [b]Degenerated, the $f$ account for this [c]Nitrodimethylaniline [d]N-Phenylpyrrole

## S1.1 Aminobenzonitrile

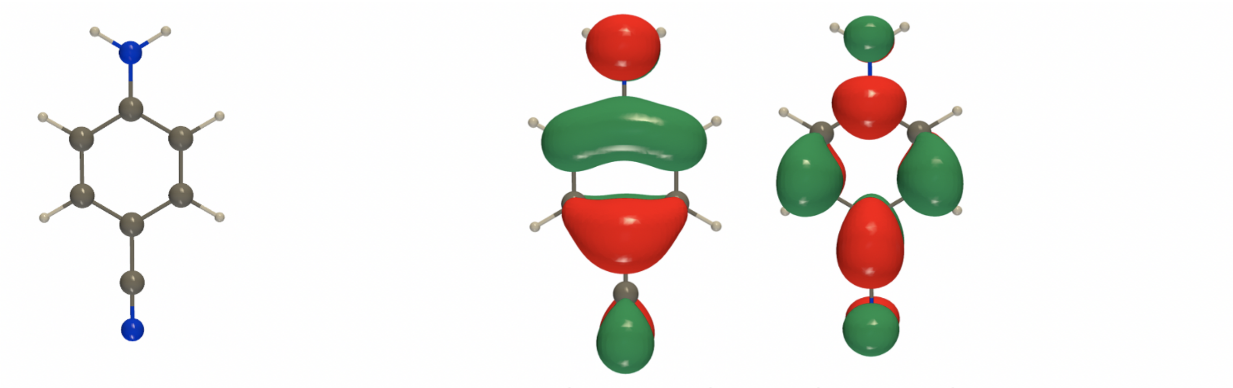

31 (HOMO, $B_1$) 32 (LUMO, $B_1$)

## S1.2 Aniline

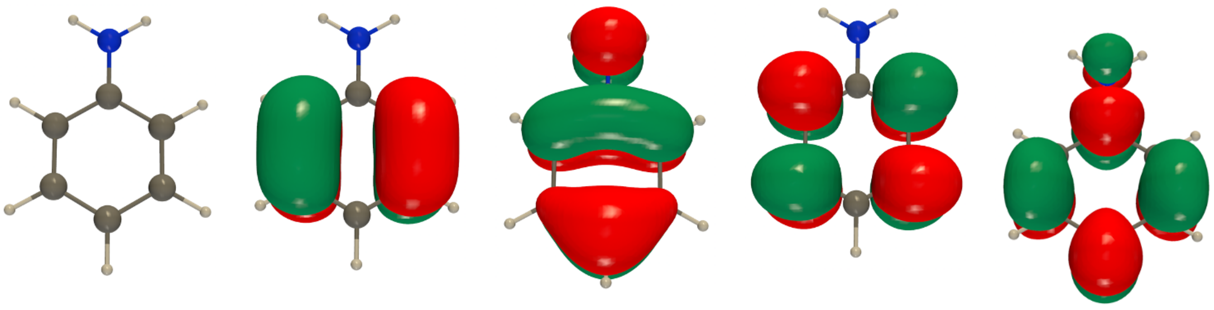

24 ($A_2$) 25 (HOMO, $B_1$) 26 (LUMO, $A_2$) 29 ($B_1$)

## S1.3 Azulene

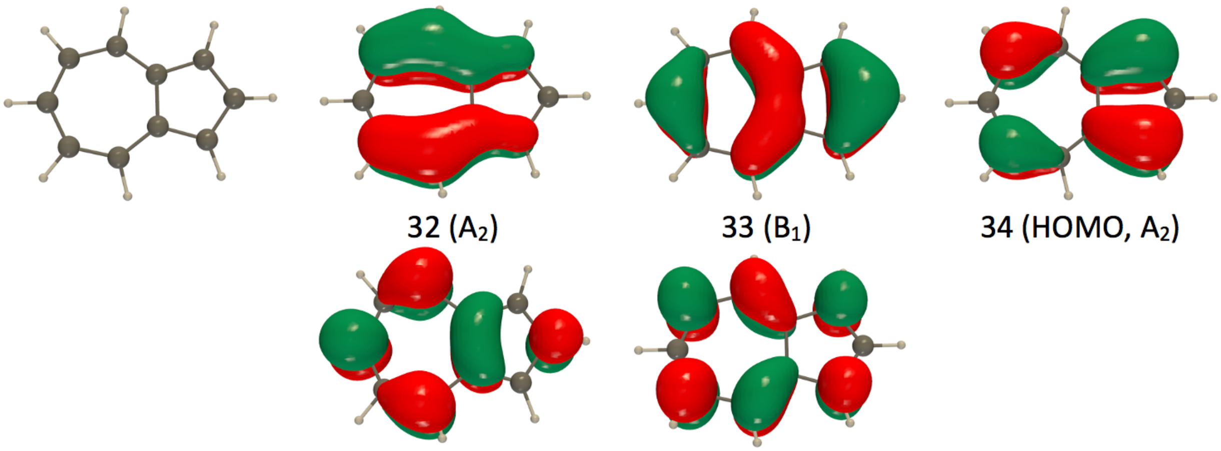

32 ($A_2$) 33 ($B_1$) 34 (HOMO, $A_2$)

35 (LUMO, $B_1$) 36 ($A_2$)

## S1.4 Benzonitrile

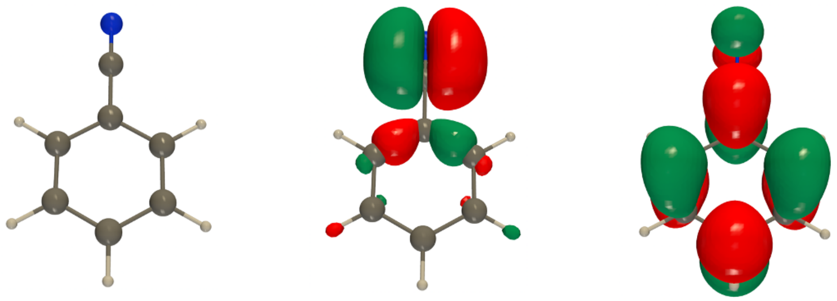

25 ($B_2$) 28 (LUMO, $B_1$)

## S1.5 Benzothiadiazole

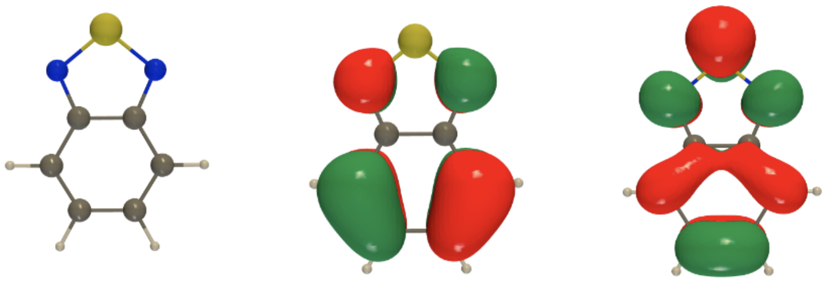

35 (HOMO, $A_2$) 36 (LUMO, $B_1$)

## S1.6 Dimethylaniline

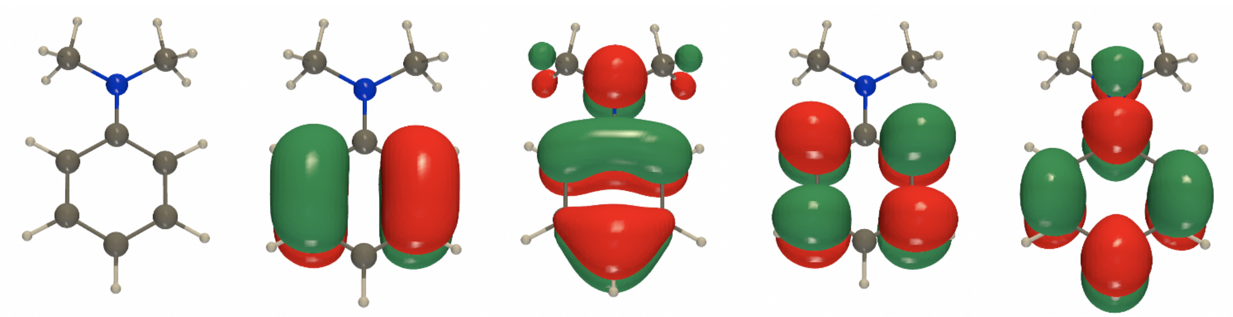

32 ($A_2$) 33 (HOMO, $B_1$) 34 (LUMO, $A_2$) 36 ($B_1$)

## S1.7 Dimethylaminobenzonitrile

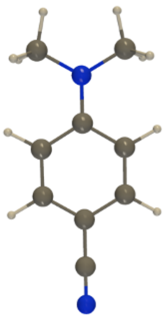

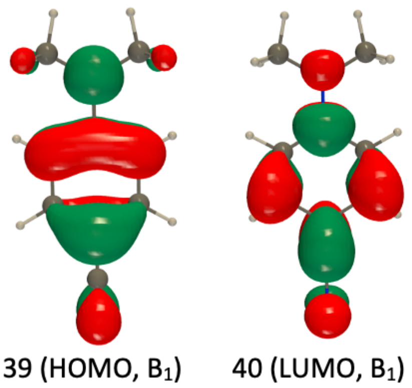


## S1.8 Dipeptide

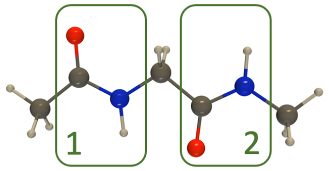


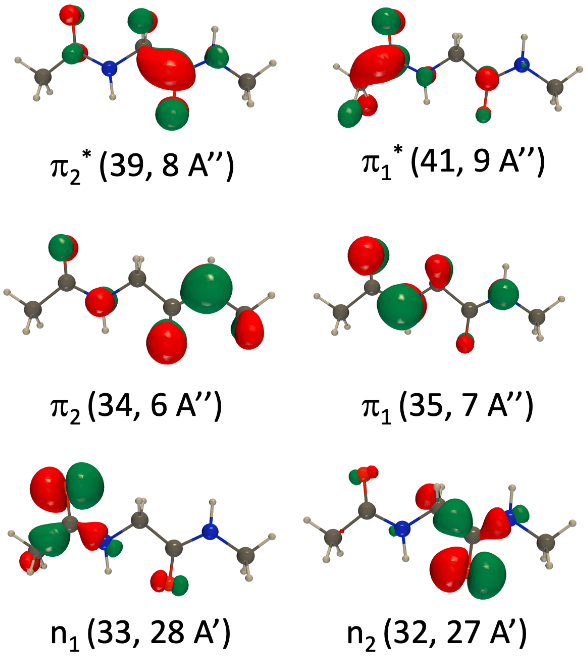

## S1.9 β-Dipeptide

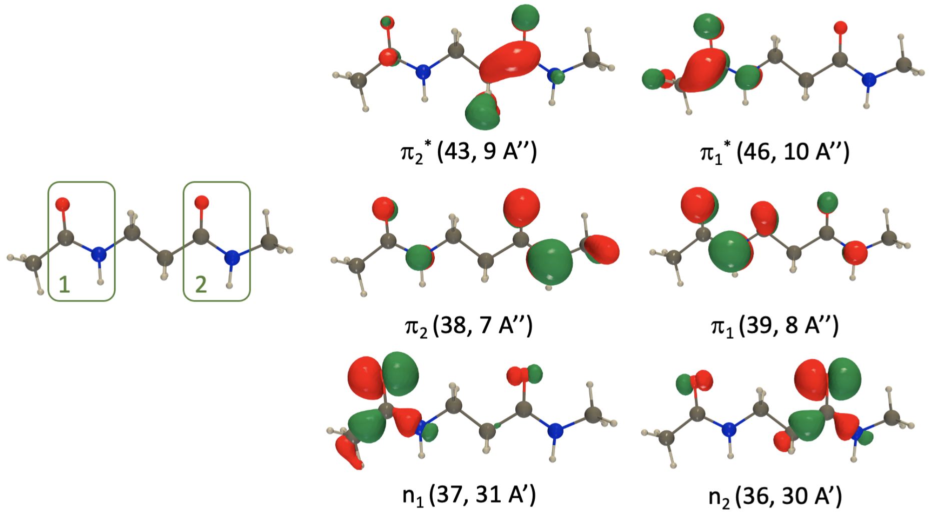


## S1.10 Hydrogen chloride

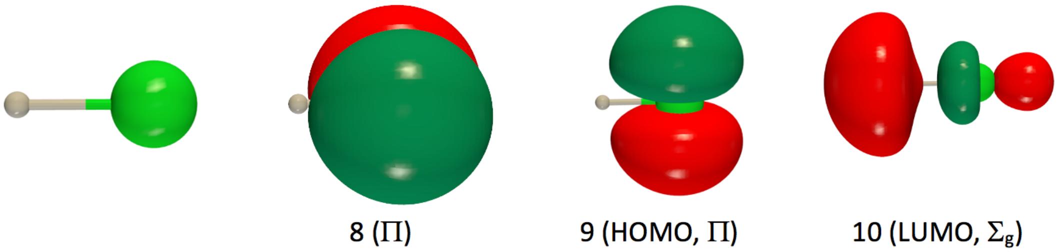


## S1.11 Nitroaniline

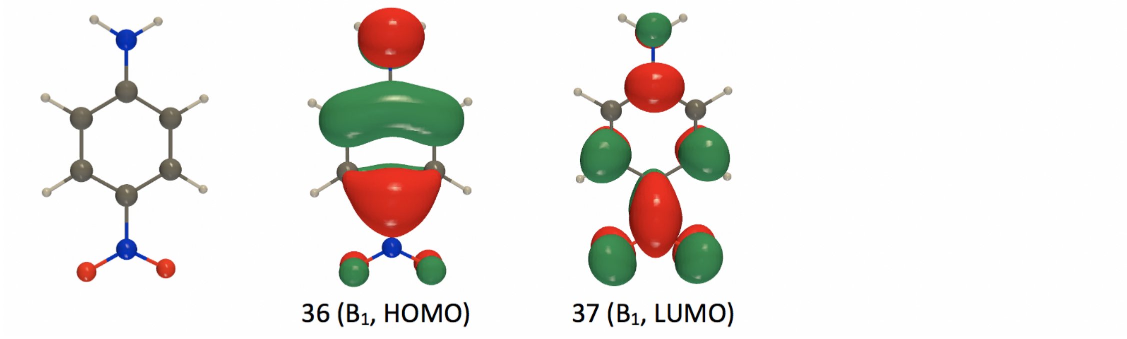

## S1.12 Nitrobenzene

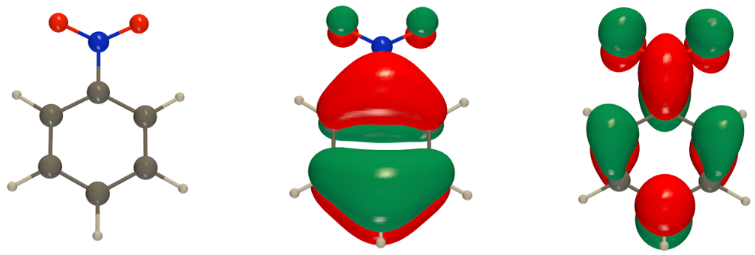

31 ($B_1$) 33 (LUMO, $B_1$)

## S1.13 Nitrodimethylaniline

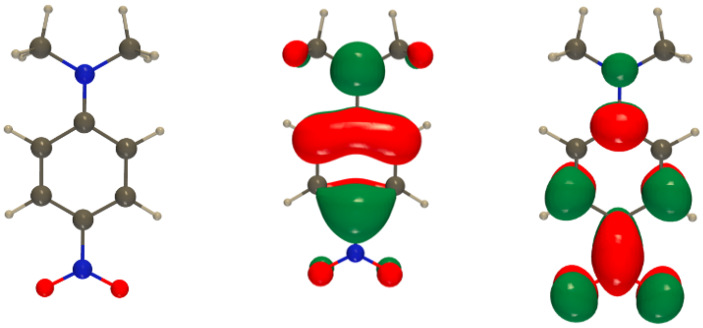

44 ($B_1$, HOMO) 45 ($B_1$, LUMO)

## S1.14 Nitropyridine N-Oxide

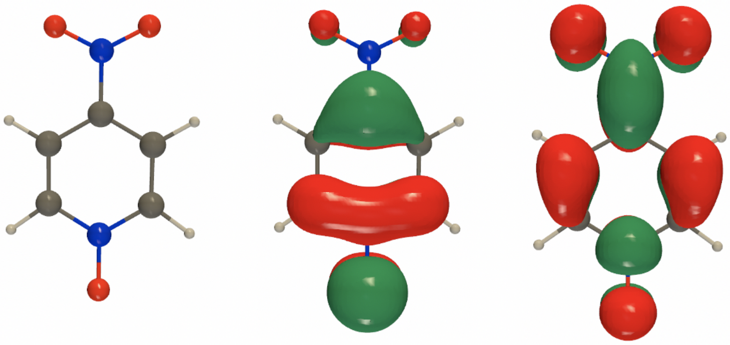

36 ($B_1$, HOMO) 37 ($B_1$, LUMO)

## S1.15 N-Phenylpyrrole

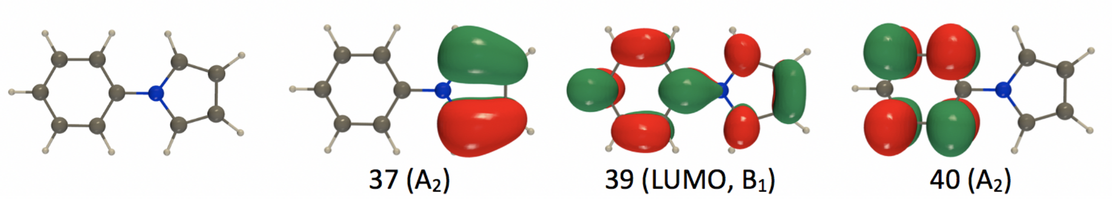


## S1.16 Phthalazine

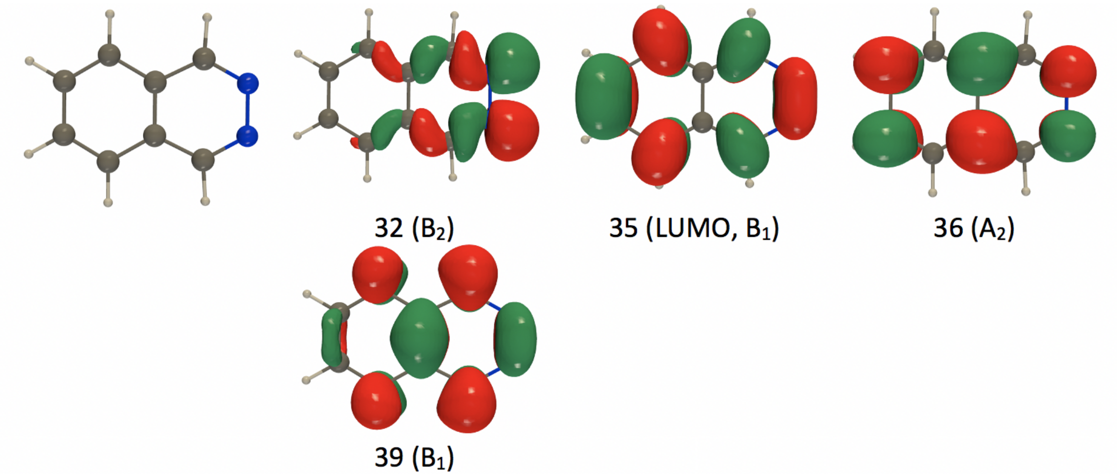


## S1.17 Quinoxaline

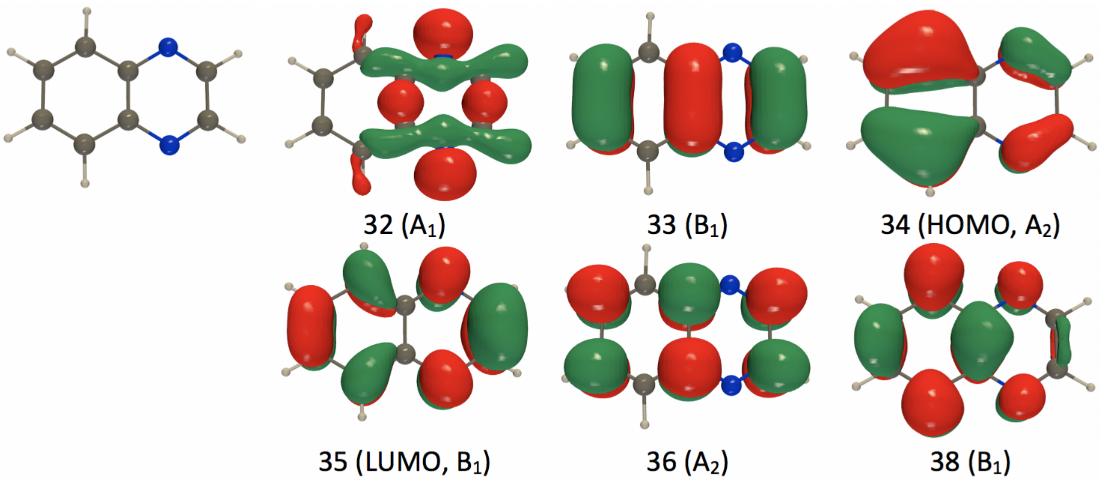

## S1.18 Twisted DMABN

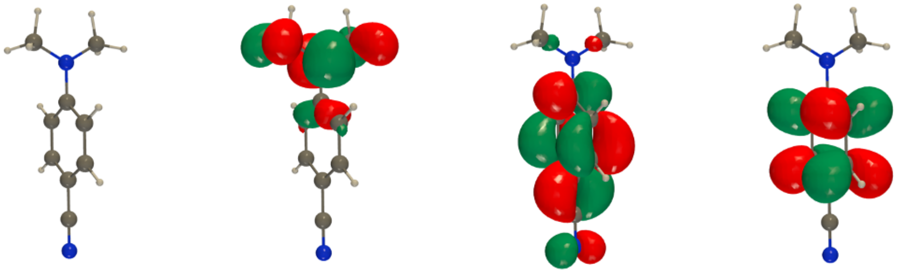

38 ($B_2$) 40 (LUMO, $B_1$) 41 ($A_2$)

## S1.19 Twisted PP

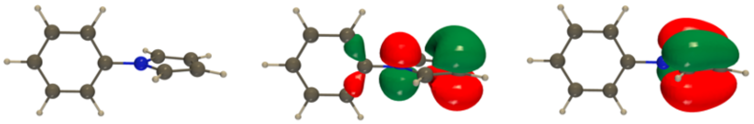

37 ($B_2$) 38 (HOMO, $A_2$)

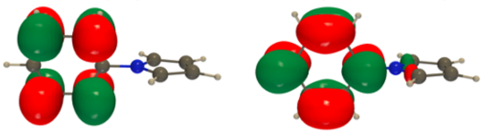

39 (LUMO, $A_2$) 40 ($B_1$)

# S2 Comparisons of CT metrics

We compare the different metrics for calculating the electron-hole average distance. At the BSE level, the $r^{\text{eh}}_{\text{BSE}}$ value is obtained as the inverse of the expectation value of the direct Coulomb interaction over the BSE eigenstates,

$$\psi^{\lambda}_{\text{BSE}}(\mathbf{r}_e, \mathbf{r}_h) = \sum_{ia} \left( X^{\lambda}_{ia} \phi_i(\mathbf{r}_h) \phi_a(\mathbf{r}_e) + Y^{\lambda}_{ia} \phi_i(\mathbf{r}_e) \phi_a(\mathbf{r}_h) \right),$$

restricting the integral to the resonant contributions,

$$1/r^{\text{eh}}_{\text{BSE}} = \sum_{ia,jb} X^{\lambda}_{ia} X^{\lambda}_{jb} (ij|ab).$$

The largest discrepancy between the BSE/ev$GW$@PBE0 and BSE/ev$GW$@HF effective $r^{\text{eh}}_{\text{BSE}}$ distances occurs for the highest CT state associated with the $\beta$-Dipeptide (transitions $S_{19}$ and $S_{18}$, respectively), namely a highly excited state for which the identification is difficult (see below). While the BSE/ev$GW$@PBE0 $S_{19}$ excitation is a clear $n_1 - \pi^*_2$ transition with well separated electron and hole densities, the BSE/ev$GW$@HF equivalent excitation contains a significant admixture of the occupied $n_2$ orbital, inducing a significant local (Frenkel) character that reduces the electron-hole average distance.

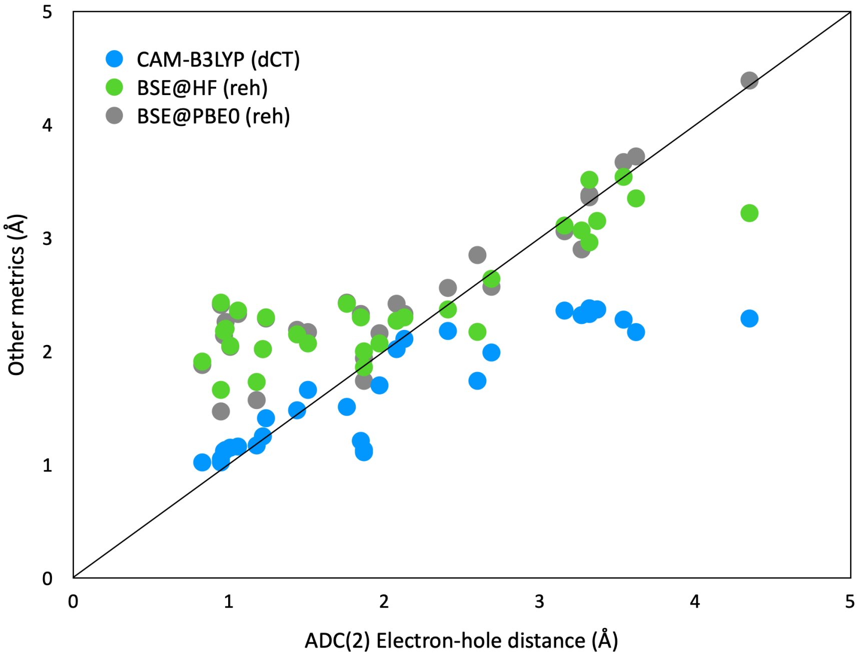


Figure S1: Comparison between CT distances as estimated by $d^{\mathrm{CT}}_{\mathrm{CAM}}$, $r^{\mathrm{eh}}_{\mathrm{BSE}}$ (using both HF and PBE0 starting orbitals), and $r^{\mathrm{eh}}_{\mathrm{ADC}}$. All values are in Å.

# S3 Results for dipeptide

In the Table below, we list many transitions determined at the EOM-CCSD and ISR-ADC(2) levels for the dipeptide. The representation of the key HF/cc-pVTZ MOs can be found in the previous pages. All virtual orbitals not represented (36, 37, 38, 40, and 42) are of Rydberg nature. From the MOs, one would expect the CT $\pi_1 \rightarrow \pi_2^\star$ transition to have a dominant 35-39 character. At both levels of theory, this corresponds to the lowest $A'$ ES, located at 7.35 eV (EOM-CCSD) and 6.98 eV [ADC(2)]. Such identification was indeed selected in Ref. 1, and seems also compatible with the original CASPT2/DZP work[2] which reported a CT at 7.18 eV, below the local $\pi \rightarrow \pi^\star$ excitations. However, it can be noted that the selected $|r_e - r_h|$ metric gives a very small charge separation of 0.09 Å for that transition. Alternatively, one could select here is a second ES in which the 35-39 contribution is dominant (at EOM-CCSD level) or large [at ADC(2) level] which is located at 8.27 eV (EOM-CCSD) and 7.66 eV [ADC(2)]. This is the transition selected by Tozer in his 2012 work,[3] and is also the one showing a large electron-hole separation of 1.55 Å according to the selected metric. In short, depending on the selected criterion, a different state would be chosen, which is a consequence of the strong mixing.

Table S2: EOM-CCSD/cc-pVTZ and ISR-ADC(2)/cc-pVTZ results for dipeptide: transition energies (in eV), oscillator strength, MO combination and nature. For the ADC(2) results, we also provide the electron-hole distance (in Å), see the main text.

| $A'$ transitions | | | | | | | | |
|---|---|---|---|---|---|---|---|---|
| EOM-CCSD/cc-pVTZ | | | | ISR-ADC(2)/cc-pVTZ | | | | |
| $\Delta E$ | $f$ | Two largest MO contributions | Nature | $\Delta E$ | $f$ | Two largest MO contributions | $\|r_e - r_h\|$ | Nature |
| 7.353 | 0.081 | 35-39 (-0.515); 34-39 (-0.288) | [a] | 6.982 | 0.091 | 35-39 (0.511); 34-39 (0.297) | 0.092 | [a] |
| 7.432 | 0.329 | 35-41 (-0.470); 34-39 (-0.311) | $\pi_1 \rightarrow \pi_1^\star$ | 7.093 | 0.268 | 35-41 (0.464); 34-39 (-0.282) | 0.628 | $\pi_1 \rightarrow \pi_1^\star$ |
| 8.025 | 0.093 | 33-37 (-0.499); 33-36 (-0.328) | Rydberg | 7.264 | 0.130 | 33-37 (-0.460); 33-36 (-0.325) | 0.678 | Rydberg |
| 8.092 | 0.060 | 35-39 (-0.328); 34-39 (0.306) | [a] | 7.408 | 0.007 | 32-36 (0.450) ; 33-37 (-0.387) | 0.912 | Rydberg |
| 8.270 | 0.034 | 32-36 (0.473); 33-37 (-0.298) | Rydberg | 7.664 | 0.092 | 34-39 (0.409); 35-39 (-0.287) | 1.554 | [a] |
| $A$" transitions | | | | | | | | |
| $\Delta E$ | $f$ | Two largest MO contributions | Nature | $\Delta E$ | $f$ | Two largest MO contributions | $\|r_e - r_h\|$ | Nature |
| 5.802 | 0.001 | 33-41 (0.498); 33-46 (0.230) | $n_1 \rightarrow \pi_1^\star$ | 5.526 | 0.001 | 33-41 (-0.498); 33-39 (-0.298) | 0.809 | $n_1 \rightarrow \pi_1^\star$ |
| 6.024 | 0.001 | 32-39 (-0.546); 32-41 (-0.213) | $n_2 \rightarrow \pi_2^\star$ | 5.735 | 0.000 | 32-39 (0.542); 32-41 (-0.208) | 0.813 | $n_2 \rightarrow \pi_2^\star$ |
| 7.224 | 0.000 | 34-36 (0.466); 35-36 (0.440) | Rydberg | 7.077 | 0.000 | 35-36 (0.463); 34-36(0.448) | 1.599 | Rydberg |
| 7.734 | 0.002 | 35-37 (0.492); 34-36 (-0.245) | Rydberg | 7.555 | 0.003 | 35-37 (0.476) ; 34-36 (-0.291) | 1.847 | Rydberg |
| 8.120 | 0.013 | 34-36 (0.304); 35-37 (0.293) | Rydberg | 7.823 | 0.000 | 33-39 (0.537); 33-41 (-0.272) | 3.617 | $n_1 \rightarrow \pi_2^\star$ |
| 8.568 | 0.040 | 34-38 (0.465); 35-38 (0.276) | Rydberg | 7.894 | 0.011 | 35-37 (-0.345); 34-36 (-0.312) | 1.204 | Rydberg |
| 8.924 | 0.000 | 33-39 (0.556); 33-41 (0.288) | $n_1 \rightarrow \pi_2^\star$ | 8.391 | 0.037 | 34-38 (0.462); 35-38 (0.286) | 0.891 | Rydberg |

[a]For these two states, the mixing is very strong, and they can be characterized either as $\pi_2 \rightarrow \pi_2^\star$ or $\pi_1 \rightarrow \pi_2^\star$

To add even more to the “confusion”, we report below the TD-CAM-B3LYP/cc-pVTZ results for the same system. It is important to note that the ordering of the MOs has changed, but the correspondence with HF is straightforward (see Figure below for Kohn-Sham orbitals). In this case, the picture is actually clearer with the lowest transition of $A'$ symmetry showing the MO nature compatible with a CT nature. It is also reflected in the metric of Le Bahers. The one-to-one mapping with the wavefunction results is however far from straightforward.

Table S3: TD-CAM-B3LYP/cc-pVTZ results for dipeptide: transition energies (in eV), oscillator strength, MO combination and nature and Le Bahers' metric results.

| | | $A'$ transitions | | | |
|---|---|---|---|---|---|
| $\Delta E$ | $f$ | Two largest MO contributions | $d^{\mathrm{CT}}$ | $q^{\mathrm{CT}}$ | Nature |
| 6.998 | 0.010 | 34-37 (0.692) | 1.699 | 0.834 | $\pi_1 \to \pi_2^\star$ |
| 7.398 | 0.301 | 34-38 (0.570); 33-37 (0.348) | 0.993 | 0.447 | $\pi_1 \to \pi_1^\star$ |
| 7.590 | 0.068 | 33-37 (0.531); 32-36 (-0.196) | 0.590 | 0.495 | $\pi_2 \to \pi_2^\star$ |
| 7.656 | 0.105 | 35-39 (0.461); 35-36 (0.446) | 0.752 | 0.960 | Rydberg |
| 7.941 | 0.008 | 35-39 (0.473); 35-36 (-0.342) | 0.624 | 0.935 | Rydberg |
| 8.132 | 0.032 | 32-36 (0.551); 35-36 (-0.246) | 1.561 | 0.937 | Rydberg |

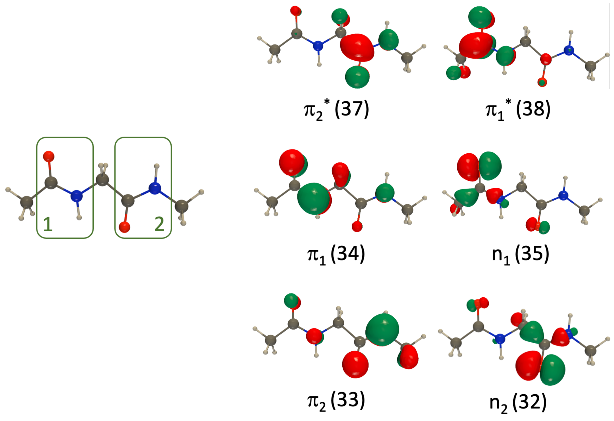


Figure S2: Key CAM-B3LYP/cc-pVTZ MOs

Coming now to BSE calculations, the partially self-consistent ev$GW$ step somehow facilitates the comparison between BSE/ev$GW$@HF and BSE/ev$GW$@PBE0 data. The BSE/ev$GW$@HF calculations are known to be less accurate but allow an easier identification with wavefunction reference techniques that build as well on HF molecular orbitals. While the HOMO, HOMO-1 and HOMO-2 levels are the $\pi_1$, $\pi_2$ and $n_1$ levels at the HF level, respectively, the corresponding ordering at the PBE0 level becomes $n_1$, $\pi_1$, $\pi_2$ due presumably

to the destabilization of the localized $n_1$ level by self-interaction. However, at the ev$GW$ level, and independently of the starting point, the ordering becomes $\pi_1$, $n_1$ and $\pi_2$, facilitating the identification between BSE/ev$GW$@HF and BSE/ev$GW$@PBE0 data. Similarly, the $\pi_2^*$ state stands at the (LUMO+1) level within both BSE/ev$GW$@HF and BSE/ev$GW$@PBE0, the HOMO being a delocalized Rydberg state (for the cc-pVTZ basis set). In both cases, the 12$^{\text{th}}$ ($S_{12}$) BSE excitation shows a clear $n_1$-$\pi_2^*$ character (see Fig. S3) with an average electron-hole distance, as defined from the direct Coulomb matrix elements, larger than any other transitions (PBE0: 3.72 Å and HF: 3.35 Å) for this system. The larger 12.35 eV HOMO-LUMO gap within ev$GW$@HF, as compared to 12.02 eV at the ev$GW$@PBE0 level, can partly explained that the $n_1$-$\pi_2^*$ CT stands 0.44 eV higher when starting with HF orbitals as compared to their PBE0 analogs.

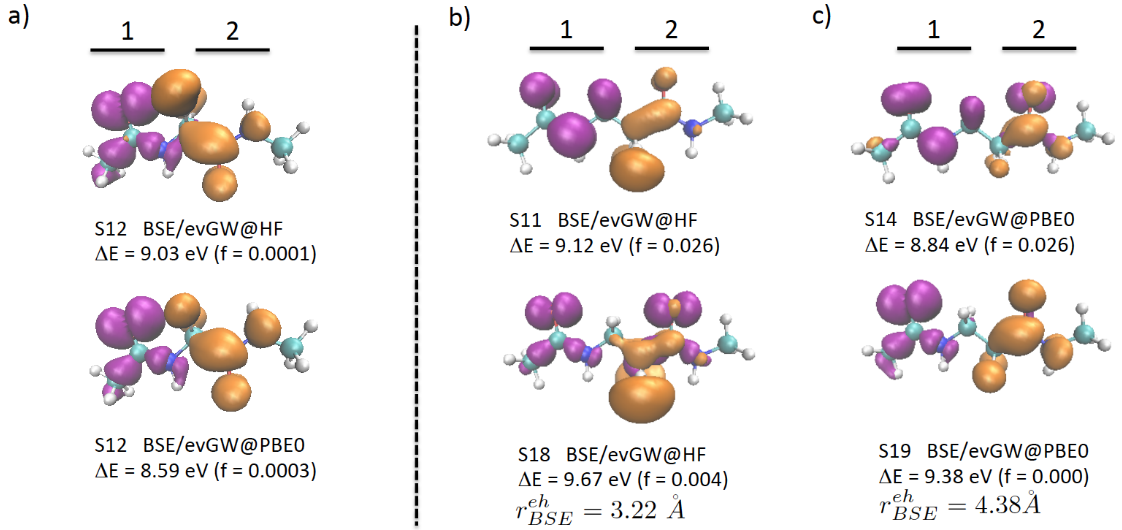


Figure S3: Plot of the hole-averaged electron distribution (orange) and electron-averaged hole distribution (purple) associated with the BSE eigenstates for (a) the Dipeptide BSE/ev$GW$@HF (top) and @PBE0 (bottom) S$_{12}$ $n_1 - \pi_2^*$ excitations , (b) the $\beta$-Dipeptide BSE/ev$GW$@HF $S_{11}$ $\pi_1 - \pi_2^*$ (top) and $S_{18}$ $n_1 - \pi_2^*$ (bottom) excitations, and (c) the $\beta$-Dipeptide BSE/ev$GW$@PBE0 $S_{14}$ $\pi_1 - \pi_2^*$ (top) and $S_{19}$ $n_1 - \pi_2^*$ (bottom) excitations.

Below, we provide a complete list of the lowest excited states of $\beta$-dipeptide, as obtained by EOM-CCSD and ISR-ADC(2). As can be seen, though the state ordering differs from one method to another, the nature of the various transitions is clearer than for the previous peptide. This holds for the CAM-B3LYP analysis as well. Concerning BSE calculations, both ev$GW$@PBE0 and ev$GW$@HF yield again a $\pi_1$, $n_1$, $\pi_2$ ordering at the top of the occupied MO levels, the $\pi_2^*$ level being the (LUMO+2) in both cases. The lowest BSE/ev$GW$@HF CT excitation ($S_{11}$) is a clear $\pi_1$-$\pi_2^*$ excitation (see Fig. S3). Such a $\pi_1$-$\pi_2^*$ excitation can be associated with the $S_{14}$ excitation in BSE/ev$GW$@PBE0 that shows however some contribution from the $n_2$ occupied MO. The BSE/ev$GW$@HF $n_1 - \pi_2^*$ excitation can be identified as the $S_{18}$ state for BSE/ev$GW$@HF, showing however a strong $n_2$ character that introduces some local character, reducing the electron-hole average distance. The corresponding BSE/ev$GW$@PBE0 state is the $S_{19}$ excitation displaying a clearer CT character and thus a much large $r^{eh}_{\text{BSE}}$.

Table S4: EOM-CCSD/cc-pVTZ and ISR-ADC(2)/cc-pVTZ results for $\beta$-Dipeptide: transition energies (in eV), oscillator strength, MO combination and nature. For the ADC(2) results, we also provide the electron-hole distance (in Å), see the main text.

| | | EOM-CCSD/cc-pVTZ | | | | ISR-ADC(2)/cc-pVTZ | | |
|---|---|---|---|---|---|---|---|---|
| | | | | $A'$ transitions | | | | |
| $\Delta E$ | $f$ | Two largest MO contributions | Nature | $\Delta E$ | $f$ | Two largest MO contributions | $\|r_e - r_h\|$ | Nature |
| 7.357 | 0.198 | 38-43 (-0.453); 38-47 (0.248) | $\pi_2 \to \pi_2^\star$ | 6.791 | 0.013 | 37-41 (-0.498); 37-40 (-0.390) | 1.446 | Rydberg |
| 7.445 | 0.229 | 39-46 (-0.456); 39-43 (-0.264) | $\pi_1 \to \pi_1^\star$ | 6.895 | 0.012 | 36-40 (0.512); 38-43 (-0.208) | 1.946 | Rydberg |
| 7.643 | 0.098 | 37-41 (-0.478); 37-40 (-0.391) | Rydberg | 7.044 | 0.250 | 38-43(0.423); 36-40 (0.288) | 0.920 | $\pi_2 \to \pi_2^\star$ |
| 7.787 | 0.030 | 36-40 (-0.581); 37-41 (0.160) | Rydberg | 7.108 | 0.273 | 39-46 (-0.466); 39-43(-0.301) | 0.643 | $\pi_1 \to \pi_1^\star$ |
| 8.832 | 0.012 | 37-45 (-0.313); 37-44 (-0.307) | Rydberg | 7.955 | 0.033 | 36-41 (0.446); 36-44 (-0.347) | 2.568 | Rydberg |
| 8.851 | 0.042 | 37-45 (0.367); 36-44 (-0.353) | Rydberg | 8.019 | 0.032 | 37-42 (0.337); 37-40 (-0.325) | 2.452 | Rydberg |
| 8.899 | 0.018 | 39-43 (0.494); 38-43 (-0.241) | $\pi_1 \to \pi_2^\star$ | 8.164 | 0.011 | 37-45 (0.561); 37-40 (0.236) | 2.242 | Rydberg |
| | | | | 8.299 | 0.004 | 39-43 (0.482); 39-46 (-0.250) | 3.155 | $\pi_1 \to \pi_2^\star$ |
| | | | | $A$" transitions | | | | |
| $\Delta E$ | $f$ | Two largest MO contributions | Nature | $\Delta E$ | $f$ | Two largest MO contributions | $\|r_e - r_h\|$ | Nature |
| 5.786 | 0.001 | 37-46 (0.512); 37-51 (-0.245) | $n_1 \to \pi_1^\star$ | 5.490 | 0.001 | 37-46 (-0.516); 37-43 (-0.239) | 0.783 | $n_1 \to \pi_1^\star$ |
| 5.860 | 0.000 | 36-43 (0.484); 36-47 (-0.291) | $n_2 \to \pi_2^\star$ | 5.565 | 0.000 | 36-43 (0.484); 36-47 (-0.284) | 0.850 | $n_2 \to \pi_2^\star$ |
| 7.032 | 0.000 | 38-40 (0.430); 39-40 (-0.351) | Rydberg | 6.863 | 0.001 | 39-40 (-0.433); 38-40 (0.344) | 1.631 | Rydberg |
| 7.091 | 0.003 | 39-41 (0.465); 39-40 (0.300) | Rydberg | 6.910 | 0.028 | 39-41 (-0.451); 38-40(-0.405) | 1.750 | Rydberg |
| 8.345 | 0.003 | 39-45 (-0.444); 39-40 (0.307) | Rydberg | 8.054 | 0.001 | 39-45 (0.348); 39-40 (0.366) | 2.228 | Rydberg |
| 8.574 | 0.019 | 38-44 (-0.436); 38-42 (0.349) | Rydberg | 8.355 | 0.003 | 38-44 (-0.434); 38-40 (0.276) | 1.385 | Rydberg |
| 8.725 | 0.017 | 39-45 (-0.391); 39-42 (-0.269) | Rydberg | 8.421 | 0.010 | 38-42 (0.468); 38-41 (-0.284) | 0.650 | Rydberg |
| 8.766 | 0.005 | 38-42 (-0.378); 38-40 (0.304) | Rydberg | 8.448 | 0.001 | 37-43 (-0.551); 37-46 (-0.198) | 4.348 | $n_1 \to \pi_2^\star$ |
| 9.299 | 0.005 | 39-44 (-0.438); 39-40 (-0.276) | Rydberg | 8.467 | 0.026 | 39-45 (0.459); 39-41(0.198) | 2.082 | Rydberg |
| 9.575 | 0.000 | 37-43 (-0.587); 37-46 (0.215) | $n_1 \to \pi_2^\star$ | | | | | |

# S4 Transferability of basis set effects

Below, we investigate the basis set effects. To do so, we compare the transition energies obtained with the same approach (e.g., CCSDT-3) and report the difference between the two basis set ($E_{\text{cc-pVTZ}} - E_{\text{cc-pVDZ}}$) considered.

Table S5: Difference between the transition energies computed with cc-pVDZ and cc-pVTZ (in eV) for CCSDT-3 and CC3.

| Compound | State | CCSDT-3 | CC3 |
|---|---|---|---|
| Aminobenzonitrile | $2\ A_1\ (\pi \to \pi^\star)$ | -0.13 | -0.13 |
| Aniline | $2\ A_1\ (\pi \to \pi^\star)$ | -0.18 | -0.18 |
| Azulene | $2\ A_1\ (\pi \to \pi^\star)$ | -0.09 | -0.09 |
| | $2\ B_2\ (\pi \to \pi^\star)$ | -0.07 | -0.07 |
| Benzonitrile | $1\ A_2\ (\pi_{\text{CN}} \to \pi^\star)$ | -0.16 | -0.16 |
| Benzothiadiazole | $1\ B_2\ (\pi \to \pi^\star)$ | -0.19 | -0.20 |
| Dimethylaminobenzonitrile | $2\ A_1\ (\pi \to \pi^\star)$ | -0.11 | -0.12 |
| Dimethylaniline | $1\ B_2\ (\pi \to \pi^\star)$ | -0.10 | -0.11 |
| | $2\ A_1\ (\pi \to \pi^\star)$ | -0.15 | -0.15 |
| Hydrogen Chloride | $1\ \Pi\ (n \to \sigma^\star)$ | -0.12 | -0.12 |
| Nitroaniline | $2\ A_1\ (\pi \to \pi^\star)$ | -0.18 | -0.19 |
| Nitrobenzene | $2\ A_1\ (\pi \to \pi^\star)$ | -0.24 | -0.25 |
| Nitrodimethylaniline | $2\ A_1\ (\pi \to \pi^\star)$ | -0.18 | -0.20 |
| Nitropyridine N-Oxide | $2\ A_1\ (\pi \to \pi^\star)$ | -0.14 | -0.16 |
| N-Phenylpyrrole | $2\ B_2\ (\pi \to \pi^\star)$ | -0.17 | -0.17 |
| | $3\ A_1\ (\pi \to \pi^\star)$ | -0.19 | -0.20 |
| Phthalazine | $1\ A_2\ (n \to \pi^\star)$ | -0.02 | -0.03 |
| | $1\ B_1\ (n \to \pi^\star)$ | -0.05 | -0.06 |
| Quinoxaline | $1\ B_2\ (\pi \to \pi^\star)$ | -0.20 | -0.21 |
| | $3\ A_1\ (\pi \to \pi^\star)$ | -0.13 | -0.14 |
| | $2\ B_1\ (n \to \pi^\star)$ | -0.11 | -0.12 |
| Twisted DMABN | $1\ A_2(n \to \pi^\star)$ | -0.06 | -0.08 |
| | $1\ B_1(n \to \pi^\star)$ | -0.13 | -0.14 |
| Twisted PP | $2\ B_2\ (\pi \to \pi^\star)$ | -0.11 | -0.12 |
| | $2\ A_1\ (\pi \to \pi^\star)$ | -0.20 | -0.21 |
| | $1\ A_2\ (\pi \to \pi^\star)$ | -0.09 | -0.11 |
| | $1\ B_1\ (\pi \to \pi^\star)$ | -0.18 | -0.18 |

Table S6: Difference between the transition energies computed with cc-pVTZ and *aug*-cc-pVTZ (in eV) for CC2, CCSD, and CCSDT-3.

| Compound | State | CC2 | CCSD | CCSDT-3 |
|---|---|---|---|---|
| Aminobenzonitrile | 2 $A_1$ ($\pi \to \pi^\star$) | -0.17 | -0.18 | -0.17 |
| Aniline | 2 $A_1$ ($\pi \to \pi^\star$) | -0.39 | -0.39 | -0.37 |
| Azulene | 2 $A_1$ ($\pi \to \pi^\star$) | -0.04 | -0.04 | |
| | 2 $B_2$ ($\pi \to \pi^\star$) | -0.04 | -0.04 | |
| Benzonitrile | 1 $A_2$ ($\pi_{\text{CN}} \to \pi^\star$) | -0.06 | -0.05 | -0.05 |
| Benzothiadiazole | 1 $B_2$ ($\pi \to \pi^\star$) | -0.07 | -0.08 | -0.07 |
| Dimethylaminobenzonitrile | 2 $A_1$ ($\pi \to \pi^\star$) | -0.07 | -0.08 | |
| Dimethylaniline | 1 $B_2$ ($\pi \to \pi^\star$) | -0.09 | -0.08 | |
| | 2 $A_1$ ($\pi \to \pi^\star$) | -0.14 | -0.14 | |
| Hydrogen Chloride | 1 $\Pi$ ($n \to \sigma^\star$) | -0.32 | -0.27 | -0.27 |
| Nitroaniline | 2 $A_1$ ($\pi \to \pi^\star$) | -0.17 | -0.17 | |
| Nitrobenzene | 2 $A_1$ ($\pi \to \pi^\star$) | -0.16 | -0.15 | -0.17 |
| Nitrodimethylaniline | 2 $A_1$ ($\pi \to \pi^\star$) | -0.16 | -0.14 | |
| Nitropyridine N-Oxide | 2 $A_1$ ($\pi \to \pi^\star$) | -0.16 | -0.14 | -0.14 |
| N-Phenylpyrrole | 2 $B_2$ ($\pi \to \pi^\star$) | -0.19 | -0.22 | |
| | 3 $A_1$ ($\pi \to \pi^\star$) | -0.16 | -0.19 | |
| Phthalazine | 1 $A_2$ ($n \to \pi^\star$) | -0.03 | -0.02 | -0.02 |
| | 1 $B_1$ ($n \to \pi^\star$) | -0.04 | -0.03 | -0.03 |
| Quinoxaline | 1 $B_2$ ($\pi \to \pi^\star$) | -0.09 | -0.10 | -0.10 |
| | 3 $A_1$ ($\pi \to \pi^\star$) | -0.09 | -0.10 | -0.09 |
| | 2 $B_1$ ($n \to \pi^\star$) | -0.15 | -0.14 | -0.13 |
| Twisted DMABN | 1 $A_2$($n \to \pi^\star$) | -0.06 | -0.06 | |
| | 1 $B_1$($n \to \pi^\star$) | -0.10 | -0.10 | |
| Twisted PP | 2 $B_2$ ($\pi \to \pi^\star$) | -0.10 | -0.15 | |
| | 2 $A_1$ ($\pi \to \pi^\star$) | -0.15 | -0.18 | |
| | 1 $A_2$ ($\pi \to \pi^\star$) | -0.09 | -0.09 | |
| | 1 $B_1$ ($\pi \to \pi^\star$) | -0.12 | -0.12 | |

# S5 Summary of the benchmark results

Table S7: MAE (eV) obtained for the full set of transition energies and the strong CT subset for all methods (see Tables 2 and 3 in the main text). We also provide the formal scaling with system size of each method where $N$ is the number of basis functions. I and P stand for the iterative and perturbative steps of the calculation, respectively. Note that the cost of the AO-to-MO integral transformation (which scales as $\mathcal{O}(N^5)$ in the general case) is not taken into account.

| Method | | Scaling | MAE | MAE (strong CT) |
|---|---|---|---|---|
| TD-DFT | $\omega$B97X-D | I-$\mathcal{O}(N^4)$ | 0.13 | 0.10 |
| | CAM-B3LYP | I-$\mathcal{O}(N^4)$ | 0.14 | 0.10 |
| | M06-2X | I-$\mathcal{O}(N^4)$ | 0.15 | 0.12 |
| | M11 | I-$\mathcal{O}(N^4)$ | 0.22 | 0.23 |
| | $\omega$B97X | I-$\mathcal{O}(N^4)$ | 0.27 | 0.35 |
| | LC-$\omega$HBPE | I-$\mathcal{O}(N^4)$ | 0.37 | 0.51 |
| | PBE0 | I-$\mathcal{O}(N^4)$ | 0.43 | 0.57 |
| | B3LYP | I-$\mathcal{O}(N^4)$ | 0.55 | 0.73 |
| BSE/ev$GW$ | @PBE0 | I-$\mathcal{O}(N^4)$ | 0.20 | 0.16 |
| | @HF | I-$\mathcal{O}(N^4)$ | 0.32 | 0.38 |
| CIS(D) | | I-$\mathcal{O}(N^4)$+P-$\mathcal{O}(N^5)$ | 0.35 | 0.37 |
| RPA(D) | | I-$\mathcal{O}(N^4)$+P-$\mathcal{O}(N^5)$ | 0.27 | 0.34 |
| CC2 | | I-$\mathcal{O}(N^5)$ | 0.12 | 0.15 |
| ADC(2) | | I-$\mathcal{O}(N^5)$ | 0.16 | 0.19 |
| EOM-MP2 | | I-$\mathcal{O}(N^5)$ | 0.53 | 0.60 |
| SOPPA | | I-$\mathcal{O}(N^5)$ | 0.62 | 0.67 |
| ADC(2.5) | | I-$\mathcal{O}(N^6)$ | 0.11 | 0.11 |
| ADC(3) | | I-$\mathcal{O}(N^6)$ | 0.25 | 0.30 |
| CCSD | | I-$\mathcal{O}(N^6)$ | 0.30 | 0.37 |
| CCSDR(3) | | I-$\mathcal{O}(N^6)$+P-$\mathcal{O}(N^7)$ | 0.08 | 0.10 |
| CCSD(T)(a)* | | I-$\mathcal{O}(N^6)$+P-$\mathcal{O}(N^7)$ | 0.10 | 0.12 |
| CC3 | | I-$\mathcal{O}(N^7)$ | 0.04 | 0.05 |
| CCSDT-3 | | I-$\mathcal{O}(N^7)$ | 0.07 | 0.09 |

# S6 Cartesian coordinates (bohrs)

## S6.1 Aminobenzonitrile – CC3(FC)/cc-pVTZ

| | | | |
|---|---|---|---|
| C | 0.00000000 | 0.00000000 | -3.36820633 |
| C | 2.27829762 | 0.00000000 | -2.01450309 |
| C | -2.27829762 | 0.00000000 | -2.01450309 |
| C | 0.00000000 | 0.00000000 | 1.93909521 |
| C | 2.27351166 | 0.00000000 | 0.59753796 |
| C | -2.27351166 | 0.00000000 | 0.59753796 |
| C | 0.00000000 | 0.00000000 | 4.63257112 |
| N | 0.00000000 | 0.00000000 | -5.94870080 |
| N | 0.00000000 | 0.00000000 | 6.83060124 |
| H | 4.04775542 | 0.00000000 | -3.02611570 |
| H | -4.04775542 | 0.00000000 | -3.02611570 |
| H | 4.03704439 | 0.00000000 | 1.61551747 |
| H | -4.03704439 | 0.00000000 | 1.61551747 |
| H | -1.62177115 | 0.00000000 | -6.91608217 |
| H | 1.62177115 | 0.00000000 | -6.91608217 |

## S6.2 Aniline – CC3(FC)/cc-pVTZ

| | | | |
|---|---|---|---|
| C | 0.00000000 | 0.00000000 | -1.78643569 |
| C | 2.27316118 | 0.00000000 | -0.43457234 |
| C | -2.27316118 | 0.00000000 | -0.43457234 |
| C | 0.00000000 | 0.00000000 | 3.53007775 |
| C | 2.26327651 | 0.00000000 | 2.18912925 |
| C | -2.26327651 | 0.00000000 | 2.18912925 |
| N | 0.00000000 | 0.00000000 | -4.38230793 |
| H | 4.03982526 | 0.00000000 | 3.18807501 |
| H | -4.03982526 | 0.00000000 | 3.18807501 |
| H | 0.00000000 | 0.00000000 | 5.56493193 |
| H | 4.04200589 | 0.00000000 | -1.45016965 |
| H | -4.04200589 | 0.00000000 | -1.45016965 |
| H | -1.62137595 | 0.00000000 | -5.34754284 |
| H | 1.62137595 | 0.00000000 | -5.34754284 |

## S6.3 Azulene – CC3(FC)/cc-pVTZ

| | | | |
|---|---|---|---|
| C | 0.00000000 | 0.00000000 | -5.08442654 |
| C | 2.16799436 | 0.00000000 | -3.55850254 |
| C | -2.16799436 | 0.00000000 | -3.55850254 |
| C | 1.40560615 | 0.00000000 | -1.02382432 |
| C | -1.40560615 | 0.00000000 | -1.02382432 |
| C | 0.00000000 | 0.00000000 | 4.72891515 |
| C | 2.38587647 | 0.00000000 | 3.61219185 |
| C | -2.38587647 | 0.00000000 | 3.61219185 |
| C | 3.00158451 | 0.00000000 | 1.05184313 |
| C | -3.00158451 | 0.00000000 | 1.05184313 |
| H | 0.00000000 | 0.00000000 | -7.11850559 |
| H | 4.09656030 | 0.00000000 | -4.20278074 |
| H | -4.09656030 | 0.00000000 | -4.20278074 |
| H | 0.00000000 | 0.00000000 | 6.77201689 |
| H | 3.96514987 | 0.00000000 | 4.90481753 |
| H | -3.96514987 | 0.00000000 | 4.90481753 |
| H | 5.00047162 | 0.00000000 | 0.61482964 |
| H | -5.00047162 | 0.00000000 | 0.61482964 |

## S6.4 Benzonitrile – CC3(FC)/cc-pVTZ

| | | | |
|---|---|---|---|
| C | 0.00000000 | 0.00000000 | -3.73018216 |
| C | 0.00000000 | 0.00000000 | -1.02720486 |
| C | 2.28760421 | 0.00000000 | 0.28592358 |
| C | -2.28760421 | 0.00000000 | 0.28592358 |
| C | 0.00000000 | 0.00000000 | 4.22270922 |
| C | 2.28059554 | 0.00000000 | 2.90986462 |
| C | -2.28059554 | 0.00000000 | 2.90986462 |
| N | 0.00000000 | 0.00000000 | -5.92640038 |
| H | 4.03930466 | 0.00000000 | -0.75078588 |
| H | -4.03930466 | 0.00000000 | -0.75078588 |
| H | 4.04556576 | 0.00000000 | 3.92452034 |
| H | -4.04556576 | 0.00000000 | 3.92452034 |
| H | 0.00000000 | 0.00000000 | 6.25892556 |

## S6.5 Benzothiadiazole – CC3(FC)/cc-pVTZ

| | | | |
|---|---|---|---|
| S | 0.00000000 | 0.00000000 | 4.12782363 |
| N | 0.00000000 | 2.37994968 | 2.16794907 |
| N | 0.00000000 | -2.37994968 | 2.16794907 |
| C | 0.00000000 | 1.35464582 | -0.15090868 |
| C | 0.00000000 | -1.35464582 | -0.15090868 |
| C | 0.00000000 | 2.70608821 | -2.46599859 |
| C | 0.00000000 | -2.70608821 | -2.46599859 |
| C | 0.00000000 | 1.34964552 | -4.66429754 |
| C | 0.00000000 | -1.34964552 | -4.66429754 |
| H | 0.00000000 | 4.74051264 | -2.44976392 |
| H | 0.00000000 | -4.74051264 | -2.44976392 |
| H | 0.00000000 | 2.32640888 | -6.45161040 |
| H | 0.00000000 | -2.32640888 | -6.45161040 |

## S6.6 Dimethylaminobenzonitrile – CCSD(T)(FC)/cc-pVTZ

| | | | |
|---|---|---|---|
| C | 0.00000000 | 0.00000000 | -1.96083197 |
| C | 2.27891314 | 0.00000000 | -0.58294740 |
| C | -2.27891314 | 0.00000000 | -0.58294740 |
| C | 0.00000000 | 0.00000000 | 3.37434994 |
| C | 2.26711046 | 0.00000000 | 2.02803761 |
| C | -2.26711046 | 0.00000000 | 2.02803761 |
| C | 0.00000000 | 0.00000000 | 6.06798788 |
| C | 2.36485177 | 0.00000000 | -5.90186899 |
| C | -2.36485177 | 0.00000000 | -5.90186899 |
| N | 0.00000000 | 0.00000000 | -4.53733249 |
| N | 0.00000000 | 0.00000000 | 8.26382999 |
| H | 4.06469412 | 0.00000000 | -1.55103579 |
| H | -4.06469412 | 0.00000000 | -1.55103579 |
| H | 4.03369195 | 0.00000000 | 3.04099978 |
| H | -4.03369195 | 0.00000000 | 3.04099978 |
| H | 1.96836611 | 0.00000000 | -7.91292844 |
| H | -1.96836611 | 0.00000000 | -7.91292844 |
| H | 3.49551175 | -1.67111709 | -5.47003452 |
| H | 3.49551175 | 1.67111709 | -5.47003452 |
| H | -3.49551175 | 1.67111709 | -5.47003452 |
| H | -3.49551175 | -1.67111709 | -5.47003452 |

## S6.7 Dimethylaniline – CCSD(T)(FC)/cc-pVTZ

| | | | |
|---|---|---|---|
| C | 0.00000000 | 0.00000000 | 4.89686867 |
| C | 2.25704297 | 0.00000000 | 3.55138467 |
| C | -2.25704297 | 0.00000000 | 3.55138467 |
| C | 2.27412639 | 0.00000000 | 0.92841898 |
| C | -2.27412639 | 0.00000000 | 0.92841898 |
| C | 0.00000000 | 0.00000000 | -0.44595239 |
| C | 2.36139267 | 0.00000000 | -4.39675011 |
| C | -2.36139267 | 0.00000000 | -4.39675011 |
| N | 0.00000000 | 0.00000000 | -3.03916783 |
| H | 4.05922248 | 0.00000000 | -0.04344476 |
| H | -4.05922248 | 0.00000000 | -0.04344476 |
| H | 4.03670718 | 0.00000000 | 4.54551891 |
| H | -4.03670718 | 0.00000000 | 4.54551891 |
| H | 0.00000000 | 0.00000000 | 6.93154996 |
| H | 1.97020408 | 0.00000000 | -6.40997108 |
| H | -1.97020408 | 0.00000000 | -6.40997108 |
| H | 3.49800498 | -1.66955347 | -3.96565000 |
| H | 3.49800498 | 1.66955347 | -3.96565000 |
| H | -3.49800498 | 1.66955347 | -3.96565000 |
| H | -3.49800498 | -1.66955347 | -3.96565000 |

## S6.8 Dipeptide

Geometry taken from Tozer's work.[4]

| | | | |
|---|---|---|---|
| C | 4.00145765 | -1.77314386 | 0.00000000 |
| C | 4.79035459 | -4.52287096 | 0.00000000 |
| C | 0.45989028 | 1.15546272 | 0.00000000 |
| C | -2.41239488 | 0.98508785 | 0.00000000 |
| C | -6.38634126 | 3.31968505 | 0.00000000 |
| O | 5.52115896 | -0.00000224 | 0.00000000 |
| O | -3.54008682 | -1.06199947 | 0.00000000 |
| N | 1.46227909 | -1.36934850 | 0.00000000 |
| N | -3.64275869 | 3.23088015 | 0.00000000 |
| H | 0.16721028 | -2.78329435 | 0.00000000 |
| H | 4.06123846 | -5.49460664 | 1.67242459 |
| H | 4.06123846 | -5.49460664 | -1.67242459 |
| H | 6.84708661 | -4.61248435 | 0.00000000 |
| H | 1.11496116 | 2.21105107 | 1.66195027 |
| H | 1.11496116 | 2.21105107 | -1.66195027 |
| H | -2.64103350 | 4.85709033 | 0.00000000 |
| H | -7.14275562 | 2.37728191 | 1.67345131 |
| H | -7.14275562 | 2.37728191 | -1.67345131 |
| H | -6.97804255 | 5.29278739 | 0.00000000 |

## S6.9 $\beta$-Dipeptide

Geometry taken from Tozer's work.[4]

| | | | |
|---|---|---|---|
| C | 6.58918038 | -4.56826263 | 0.00000000 |
| C | 5.17362360 | -2.07948430 | 0.00000000 |
| C | 1.04705727 | 0.01942326 | 0.00000000 |
| C | -1.72819038 | -0.71776460 | 0.00000000 |
| C | -3.43041309 | 1.60135838 | 0.00000000 |
| C | -7.86580376 | 3.03336026 | 0.00000000 |
| O | 6.27324370 | -0.02495897 | 0.00000000 |
| O | -2.57942355 | 3.77041689 | 0.00000000 |
| N | -5.95554949 | 1.06846646 | 0.00000000 |
| N | 2.60158240 | -2.24787031 | 0.00000000 |
| H | 5.35359766 | -6.22320108 | 0.00000000 |
| H | 7.80657234 | -4.63500699 | 1.66518935 |
| H | 7.80657234 | -4.63500699 | -1.66518935 |
| H | 1.76369472 | -3.96316714 | 0.00000000 |
| H | 1.48693132 | 1.17659249 | 1.65410371 |
| H | 1.48693132 | 1.17659249 | -1.65410371 |
| H | -2.16358152 | -1.87414506 | 1.66716097 |
| H | -2.16358152 | -1.87414506 | -1.66716097 |
| H | -6.50845000 | -0.76021979 | 0.00000000 |
| H | -6.87365297 | 4.83685836 | 0.00000000 |
| H | -9.05737065 | 2.91279080 | 1.68423593 |
| H | -9.05737065 | 2.91279080 | -1.68423593 |

## S6.10 Hydrogen chloride (HCl) – CC3(full)/*aug*-cc-pVTZ

| | | | |
|---|---|---|---|
| H | 0.00000000 | 0.00000000 | 2.38483140 |
| Cl | 0.00000000 | 0.00000000 | -0.02489783 |

## S6.11 Nitroaniline (pNA) – CC3(FC)/cc-pVTZ

| | | | |
|---|---|---|---|
| C | 0.00000000 | 0.00000000 | -4.05915738 |
| C | 2.28068352 | 0.00000000 | -2.70811066 |
| C | -2.28068352 | 0.00000000 | -2.70811066 |
| C | 0.00000000 | 0.00000000 | 1.19144079 |
| C | 2.28308329 | 0.00000000 | -0.09681843 |
| C | -2.28308329 | 0.00000000 | -0.09681843 |
| N | 0.00000000 | 0.00000000 | 3.94052757 |
| N | 0.00000000 | 0.00000000 | -6.63741535 |
| O | 2.04948184 | 0.00000000 | 5.01410797 |
| O | -2.04948184 | 0.00000000 | 5.01410797 |
| H | 4.04799128 | 0.00000000 | -3.72195018 |
| H | -4.04799128 | 0.00000000 | -3.72195018 |
| H | 4.02032559 | 0.00000000 | 0.95557275 |
| H | -4.02032559 | 0.00000000 | 0.95557275 |
| H | -1.62132329 | 0.00000000 | -7.60488781 |
| H | 1.62132329 | 0.00000000 | -7.60488781 |

## S6.12 Nitrobenzene – CC3(FC)/cc-pVTZ

| | | | |
|---|---|---|---|
| C | 0.00000000 | 0.00000000 | -0.33719774 |
| C | 2.29667056 | 0.00000000 | 0.92138137 |
| C | -2.29667056 | 0.00000000 | 0.92138137 |
| C | 0.00000000 | 0.00000000 | 4.85826496 |
| C | 2.28247086 | 0.00000000 | 3.54756893 |
| C | -2.28247086 | 0.00000000 | 3.54756893 |
| N | 0.00000000 | 0.00000000 | -3.11429157 |
| O | -2.05476165 | 0.00000000 | -4.18095202 |
| O | 2.05476165 | 0.00000000 | -4.18095202 |
| H | 4.02347357 | 0.00000000 | -0.14769848 |
| H | -4.02347357 | 0.00000000 | -0.14769848 |
| H | 4.04624818 | 0.00000000 | 4.56388578 |
| H | -4.04624818 | 0.00000000 | 4.56388578 |
| H | 0.00000000 | 0.00000000 | 6.89454456 |

## S6.13 Nitrodimethylaniline – CCSD(T)(FC)/cc-pVTZ

| | | | |
|---|---|---|---|
| C | 0.00000000 | 0.00000000 | -2.70893747 |
| C | 2.28286889 | 0.00000000 | -1.33300281 |
| C | -2.28286889 | 0.00000000 | -1.33300281 |
| C | 0.00000000 | 0.00000000 | 2.57206374 |
| C | 2.27821428 | 0.00000000 | 1.27798588 |
| C | -2.27821428 | 0.00000000 | 1.27798588 |
| C | 2.36504204 | 0.00000000 | -6.64945038 |
| C | -2.36504204 | 0.00000000 | -6.64945038 |
| N | 0.00000000 | 0.00000000 | -5.28314977 |
| N | 0.00000000 | 0.00000000 | 5.31851989 |
| O | 2.04957627 | 0.00000000 | 6.39360902 |
| O | -2.04957627 | 0.00000000 | 6.39360902 |
| H | 4.06683325 | 0.00000000 | -2.30372191 |
| H | -4.06683325 | 0.00000000 | -2.30372191 |
| H | 4.01906768 | 0.00000000 | 2.32551175 |
| H | -4.01906768 | 0.00000000 | 2.32551175 |
| H | 1.96723800 | 0.00000000 | -8.66013185 |
| H | -1.96723800 | 0.00000000 | -8.66013185 |
| H | 3.49498309 | -1.67118066 | -6.21739275 |
| H | 3.49498309 | 1.67118066 | -6.21739275 |
| H | -3.49498309 | 1.67118066 | -6.21739275 |
| H | -3.49498309 | -1.67118066 | -6.21739275 |

## S6.14 Nitropyridine N-Oxide – CCSD(T)(FC)/cc-pVTZ

| | | | |
|---|---|---|---|
| C | 0.00000000 | 0.00000000 | -1.21738204 |
| C | 2.26825255 | 0.00000000 | 0.09038008 |
| C | -2.26825255 | 0.00000000 | 0.09038008 |
| C | 2.22988276 | 0.00000000 | 2.68605086 |
| C | -2.22988276 | 0.00000000 | 2.68605086 |
| N | 0.00000000 | 0.00000000 | -3.96704616 |
| N | 0.00000000 | 0.00000000 | 4.00601244 |
| O | 0.00000000 | 0.00000000 | 6.38961931 |
| O | -2.05398155 | 0.00000000 | -5.02438491 |
| O | 2.05398155 | 0.00000000 | -5.02438491 |
| H | 4.03491913 | 0.00000000 | -0.90939267 |
| H | -4.03491913 | 0.00000000 | -0.90939267 |
| H | 3.88274506 | 0.00000000 | 3.86446617 |
| H | -3.88274506 | 0.00000000 | 3.86446617 |

## S6.15 N-Phenylpyrrole – CCSD(T)(FC)/cc-pVTZ

| | | | |
|---|---|---|---|
| C | 0.00000000 | 0.00000000 | 0.78511855 |
| C | 2.26951425 | 0.00000000 | 2.12513335 |
| C | -2.26951425 | 0.00000000 | 2.12513335 |
| C | 0.00000000 | 0.00000000 | 6.08505036 |
| C | 2.26188550 | 0.00000000 | 4.74952804 |
| C | -2.26188550 | 0.00000000 | 4.74952804 |
| C | 2.11189435 | 0.00000000 | -3.40622062 |
| C | -2.11189435 | 0.00000000 | -3.40622062 |
| C | 1.34457992 | 0.00000000 | -5.87759851 |
| C | -1.34457992 | 0.00000000 | -5.87759851 |
| N | 0.00000000 | 0.00000000 | -1.87596109 |
| H | 4.04529764 | 0.00000000 | 1.13844406 |
| H | -4.04529764 | 0.00000000 | 1.13844406 |
| H | 4.03918748 | 0.00000000 | 5.74456463 |
| H | -4.03918748 | 0.00000000 | 5.74456463 |
| H | 0.00000000 | 0.00000000 | 8.12006610 |
| H | 3.97993856 | 0.00000000 | -2.63372956 |
| H | -3.97993856 | 0.00000000 | -2.63372956 |
| H | 2.56993408 | 0.00000000 | -7.49221560 |
| H | -2.56993408 | 0.00000000 | -7.49221560 |

## S6.16 Phthalazine – CC3(FC)/cc-pVTZ

| | | | |
|---|---|---|---|
| C | 0.00000000 | 1.32459443 | -0.07132677 |
| C | 0.00000000 | -1.32459443 | -0.07132677 |
| C | 0.00000000 | 2.65486490 | -2.37693013 |
| C | 0.00000000 | -2.65486490 | -2.37693013 |
| C | 0.00000000 | 1.33510515 | -4.61541123 |
| C | 0.00000000 | -1.33510515 | -4.61541123 |
| C | 0.00000000 | 2.49806192 | 2.33813333 |
| C | 0.00000000 | -2.49806192 | 2.33813333 |
| N | 0.00000000 | 1.29575320 | 4.50170701 |
| N | 0.00000000 | -1.29575320 | 4.50170701 |
| H | 0.00000000 | 4.69409431 | -2.36246981 |
| H | 0.00000000 | -4.69409431 | -2.36246981 |
| H | 0.00000000 | 2.33538579 | -6.38945264 |
| H | 0.00000000 | -2.33538579 | -6.38945264 |
| H | 0.00000000 | 4.53863166 | 2.46976178 |
| H | 0.00000000 | -4.53863166 | 2.46976178 |

## S6.17 Quinoxaline – CC3(FC)/cc-pVTZ

| | | | |
|---|---|---|---|
| C | 0.00000000 | 1.33833541 | 0.04624026 |
| C | 0.00000000 | -1.33833541 | 0.04624026 |
| C | 0.00000000 | 2.65319151 | -2.27752466 |
| C | 0.00000000 | -2.65319151 | -2.27752466 |
| C | 0.00000000 | 1.33717941 | -4.51073479 |
| C | 0.00000000 | -1.33717941 | -4.51073479 |
| C | 0.00000000 | 1.33936683 | 4.32768896 |
| C | 0.00000000 | -1.33936683 | 4.32768896 |
| N | 0.00000000 | 2.68409862 | 2.24219152 |
| N | 0.00000000 | -2.68409862 | 2.24219152 |
| H | 0.00000000 | 4.68915946 | -2.22328575 |
| H | 0.00000000 | -4.68915946 | -2.22328575 |
| H | 0.00000000 | 2.33972888 | -6.28367426 |
| H | 0.00000000 | -2.33972888 | -6.28367426 |
| H | 0.00000000 | 2.35369837 | 6.10018213 |
| H | 0.00000000 | -2.35369837 | 6.10018213 |

## S6.18 Twisted Dimethylaniline – CCSD(T)(FC)/cc-pVTZ

| | | | |
|---|---|---|---|
| C | 0.00000000 | 0.00000000 | -1.92629020 |
| C | 2.27225178 | 0.00000000 | -0.58317962 |
| C | -2.27225178 | 0.00000000 | -0.58317962 |
| C | 0.00000000 | 0.00000000 | 3.35560653 |
| C | 2.28330254 | 0.00000000 | 2.03752961 |
| C | -2.28330254 | 0.00000000 | 2.03752961 |
| C | 0.00000000 | 0.00000000 | 6.05799119 |
| C | 0.00000000 | 2.39191725 | -5.88267373 |
| C | 0.00000000 | -2.39191725 | -5.88267373 |
| N | 0.00000000 | 0.00000000 | -4.58434634 |
| N | 0.00000000 | 0.00000000 | 8.25212738 |
| H | 4.02777860 | 0.00000000 | -1.61674521 |
| H | -4.02777860 | 0.00000000 | -1.61674521 |
| H | 4.03804248 | 0.00000000 | 3.06961213 |
| H | -4.03804248 | 0.00000000 | 3.06961213 |
| H | 0.00000000 | 2.05258096 | -7.90903256 |
| H | 0.00000000 | -2.05258096 | -7.90903256 |
| H | 1.66857920 | 3.52919279 | -5.43615170 |
| H | -1.66857920 | 3.52919279 | -5.43615170 |
| H | -1.66857920 | -3.52919279 | -5.43615170 |
| H | 1.66857920 | -3.52919279 | -5.43615170 |

## S6.19 Twisted N-Phenylpyrrole – CCSD(T)(FC)/cc-pVTZ

| | | | |
|---|---|---|---|
| C | 0.00000000 | 0.00000000 | 0.80351712 |
| C | 2.28073444 | 0.00000000 | 2.10816686 |
| C | -2.28073444 | 0.00000000 | 2.10816686 |
| C | 0.00000000 | 0.00000000 | 6.05091031 |
| C | 2.27731959 | 0.00000000 | 4.73583348 |
| C | -2.27731959 | 0.00000000 | 4.73583348 |
| C | 0.00000000 | 2.11496090 | -3.38187966 |
| C | 0.00000000 | -2.11496090 | -3.38187966 |
| C | 0.00000000 | 1.34265418 | -5.86240596 |
| C | 0.00000000 | -1.34265418 | -5.86240596 |
| N | 0.00000000 | 0.00000000 | -1.87814812 |
| H | 4.02558097 | 0.00000000 | 1.05801658 |
| H | -4.02558097 | 0.00000000 | 1.05801658 |
| H | 4.04316226 | 0.00000000 | 5.75023395 |
| H | -4.04316226 | 0.00000000 | 5.75023395 |
| H | 0.00000000 | 0.00000000 | 8.08702673 |
| H | 0.00000000 | 3.96297102 | -2.54995976 |
| H | 0.00000000 | -3.96297102 | -2.54995976 |
| H | 0.00000000 | 2.56243264 | -7.48144109 |
| H | 0.00000000 | -2.56243264 | -7.48144109 |

# References


(1) Casanova-Páez, M.; Dardis, M. B.; Goerigk, L. $\omega$B2PLYP and $\omega$B2GPPLYP: The First Two Double-Hybrid Density Functionals with Long-Range Correction Optimized for Excitation Energies. *J. Chem. Theory Comput.* **2019**, *15*, 4735–4744.

(2) Serrano-Andrés, L.; Fülscher, M. P. Theoretical Study of the Electronic Spectroscopy of Peptides. III. Charge-Transfer Transitions in Polypeptides. *J. Am. Chem. Soc.* **1998**, *120*, 10912–10920.

(3) Peach, M. J. G.; Tozer, D. J. Overcoming Low Orbital Overlap and Triplet Instability Problems in TDDFT. *J. Phys. Chem. A* **2012**, *116*, 9783–9789.

(4) Peach, M. J. G.; Benfield, P.; Helgaker, T.; Tozer, D. J. Excitation Energies in Density Functional Theory: an Evaluation and a Diagnostic Test. *J. Chem. Phys.* **2008**, *128*, 044118.
